# Supplementary material for: Understanding Information Disclosure from Secure Computation Output: A Study of Average Salary Computation
Source: arXiv:2209.10457 source file (2024-03-21)
Supplement: Supplementary file 1 [file appendix.tex]

\appendix

\section{Additional Proofs}
\label{sec:additional_proofs}

\begin{proof}[Proof of Claim~\ref{claim4}]
  \proofthree
\end{proof}

\threeExec
